# Supplementary material for: Shattered Time: Can a Dissipative Time Crystal Survive Many-Body Correlations?
Source: arXiv:1805.03343 ancillary file (2019-01-18)
Supplement: Supplementary file 1 [file Shattered_Time_SM.pdf]

# Supplemental Material:
# Shattered Time: Can a Dissipative Time Crystal Survive Many-Body Correlations?

K. Tucker,[1,2] B. Zhu,[1,3,4] R. J. Lewis-Swan,[1,3] J. Marino,[1,3,5] F. Jimenez,[2] J. G. Restrepo,[2] and A. M. Rey[1,3]

[1]*JILA, NIST, Department of Physics, University of Colorado, Boulder, CO 80309, USA*
[2]*Department of Applied Mathematics, University of Colorado, Boulder, CO 80309, USA*
[3]*Center for Theory of Quantum Matter, University of Colorado, Boulder, CO 80309, USA*
[4]*ITAMP, Harvard-Smithsonian Center for Astrophysics, Cambridge, MA 02138, USA*
[5]*Department of Physics, Harvard University, Cambridge MA, 02138, USA*

(Dated: June 29, 2018)

## I. INTRODUCTION

The dynamics of the system described in the main text are given by the following master equation for the density operator $\hat{\rho}$:

$$\begin{aligned}\frac{d\hat{\rho}}{dt} =& i\sum_a [\frac{\delta_a}{2}\hat{\sigma}_a^z, \hat{\rho}] - i\Gamma\sum_{a\neq b} g[\hat{\sigma}_a^+\hat{\sigma}_b^-, \hat{\rho}] \\ &-\frac{\Gamma}{2}\sum_{a,b} f(\{\hat{\sigma}_a^+\hat{\sigma}_b^-, \hat{\rho}\} - 2\hat{\sigma}_b^-\hat{\rho}\hat{\sigma}_a^+) - \frac{W}{2}\sum_a(\{\hat{\sigma}_a^-\hat{\sigma}_a^+, \hat{\rho}\} - 2\hat{\sigma}_a^+\hat{\rho}\hat{\sigma}_a^-). \end{aligned} \quad \text{(S1)}$$

Here we have dropped self-interaction in the second sum because it gives rise to a negligible single particle term that can be removed by moving to an appropriate rotating frame. Equations of motion for the expectation of a particular observable $\hat{\Omega}$ can be derived from the master equation according to the expression

$$\frac{d}{dt}\langle\hat{\Omega}\rangle = \frac{d}{dt}\mathrm{Tr}\left[\hat{\Omega}\hat{\rho}\right] = \mathrm{Tr}\left[\hat{\Omega}\frac{d\hat{\rho}}{dt}\right],$$

assuming $\hat{\Omega}$ has no explicit time dependence. The density operator $\hat{\rho}$ in the above is a $2^N \times 2^N$ complex valued matrix. The exponential scaling of the size of the density matrix with the number of particles makes exact solutions to the master equation inaccessible for $N \gtrsim 16$. In what follows, we examine the various approaches we have taken to address this issue and also provide detailed derivations of results mentioned in the main text.

We first examine the mean-field approximation and associated results. Next, we look beyond the mean-field to a second order cumulant expansion that allows for the modeling of both disorder and many-body correlations. Finally, we derive results for mutual information growth and explore its relationship with eigenvalues of the Liouvillian operator in the master equation.

## II. MEAN-FIELD

### A. Equations

In a mean-field approach, we assume that the many-body density matrix of the system can be factorized as the tensor product of single site density matrices. The components of the single site density matrix $\hat{\rho}_a$ can be visualized as a Bloch vector, $\vec{\mathcal{S}}_a = \{R_a\cos\phi_a,\, R_a\sin\phi_a,\, s_a\}$. This approach results in the system of $3N$ coupled ordinary differential equations

$$\begin{aligned}\frac{ds_a}{dt} &= -\Gamma R_a\sum_{b\neq a} R_b\left[f\cos(\phi_b-\phi_a) + 2g\sin(\phi_b-\phi_a)\right] \\ &\quad - f\Gamma\left(\frac{1}{2}+s_a\right) + W\left(\frac{1}{2}-s_a\right), \\ \frac{dR_a}{dt} &= -\frac{(f\Gamma+W)}{2}R_a + \Gamma s_a\sum_{b\neq a} R_b\left[f\cos(\phi_b-\phi_a) + 2g\sin(\phi_b-\phi_a)\right], \\ \frac{d\phi_a}{dt} &= -\delta_a + \frac{\Gamma s_a}{R_a}\sum_{b\neq a} R_b\left[f\sin(\phi_b-\phi_a) - 2g\cos(\phi_b-\phi_a)\right]. \end{aligned} \quad \text{(S2)}$$

The equation that determines the evolution of the phase $\phi_a$ is remarkably similar to the Sakaguchi-Kuramoto model for synchronization of phase oscillators [S1], which can be written as

$$\frac{d\phi_a}{dt} = \delta_a + \sum_{b\neq a} \left[ f \sin(\phi_b - \phi_a) - g \cos(\phi_b - \phi_a) \right]. \tag{S3}$$

While the evolution of the phases in Eq. (S2) is coupled to the other dynamical variables, we find that our model also supports synchronized solutions.

To study the collective dynamics, we define the order parameter $S^+ = \sum_a R_a e^{i\phi_a} = NZe^{-i\omega_{\rm MF}t}$, and focus on its normalized magnitude $Z$ and frequency $\omega_{\rm MF}$. First we will consider the case of identical frequencies, finding that elastic interactions break the time symmetry and induce oscillations with a frequency $\omega_{\rm MF}$ proportional to $g$. Then we consider the robustness of these results against disorder. In particular, we show that when the oscillator frequencies $\delta_a$ are heterogeneous and $N \gg 1$, the global oscillation frequency $\omega_{\rm MF}$ is the same as the one found for identical frequencies.

### B. Homogeneous System

First we consider the case of no disorder, i.e., $\delta_a = 0$ (note that, by moving to a rotating frame, one can assume without loss of generality that $\delta_a = \delta = 0$). This part follows the analysis done in Ref. [S2]. Since all the oscillators are identical, one can look for a stationary rotating solution in which $\phi_a = \omega_{\rm MF}t$, $R_a = R, \dot{R} = 0$, $s_a = s, \dot{s} = 0$. This gives

$$s = \frac{f\Gamma + W}{2fN\Gamma}, \tag{S4}$$

$$R = \frac{\sqrt{fN\Gamma(W - f\Gamma) - (f\Gamma + W)^2}}{\sqrt{2}fN\Gamma}, \tag{S5}$$

$$\omega_{\rm MF} = \frac{g(f\Gamma + W)}{f}, \tag{S6}$$

and, in this case, we have $Z = R$. The order parameter is nonzero only when $fN\Gamma(W - \Gamma) - (f\Gamma + W)^2 > 0$, which occurs in the finite range $N - 2 - \sqrt{N^2 - 8N} < 2W/(f\Gamma) < N - 2 + \sqrt{N^2 - 8N}$. For $N \gg 1$, this simplifies to $f\Gamma < W < fN\Gamma$. In particular, we note that when $W < f\Gamma$ there is no positive solution. Thus, only intermediate values of pumping can bring the system to a synchronized state. There is a synchronized solution (i.e., $Z > 0$) only if $N \geq 8$, corresponding to an onset at $W = 3f\Gamma$.

In the following we focus on the *optimal pumping* value $W_{opt}$ at which the order parameter achieves a maximum. In the thermodynamic limit, the optimal pumping is given by

$$W_{opt} = \frac{fN\Gamma}{2}. \tag{S7}$$

At optimal pumping, the oscillation frequency is

$$\omega_{\rm MF} = \frac{gN\Gamma}{2}, \tag{S8}$$

and the order parameter takes the value $Z_{opt} = 1/\sqrt{8}$.

### C. Disorder

Now we consider the effect of a heterogeneous frequency distribution on the time crystal. In particular, we are interested in the robustness of the oscillation frequency. To this end, we first rewrite Eqs. (S2) in terms of the order parameter $Ze^{i\psi} = \sum_a R_a e^{i\phi_a}/N$, assuming $N \gg 1$:

$$\dot{s}_a = -fN\Gamma R_a Z\cos(\psi - \phi_a) - 2gN\Gamma R_a Z \sin(\psi - \phi_a) + W\left(\frac{1}{2} - s_a\right) - f\Gamma\left(\frac{1}{2} + s_a\right), \tag{S9}$$

$$\dot{R}_a = -\frac{(W + f\Gamma)}{2}R_a + fNs_a\Gamma Z\cos(\psi - \phi_a) + 2gNs_a\Gamma Z\sin(\psi - \phi_a), \tag{S10}$$

$$\dot{\phi}_a = -\delta_a - \frac{2s_a gNZ\Gamma}{R_a}\cos(\psi - \phi_a) + \frac{s_a fNZ\Gamma}{R_a}\sin(\psi - \phi_a). \tag{S11}$$

Now we look for steady rotating solutions of Eqs. (S2) of the form $\phi_a = \psi - \theta_a$, with $R_a$, $s_a$, and $\theta_a$ constant, and $\dot{\psi} = \omega_{\rm MF}$. Inserting this Ansatz in Eqs. (S9), solving for $R_a$, $s_a$, and $\theta_a$, and requiring the self-consistent conditions

$$Z = \sum_a R_a \cos(\theta_a), \tag{S12}$$

$$0 = \sum_a R_a \sin(\theta_a), \tag{S13}$$

we obtain

$$Z = \frac{1}{N}\sum_{a=1}^{N} \frac{Z\Gamma(W-\Gamma f)(Nf(\Gamma f+W) - 4Ng(\delta_a+\omega_{\rm MF}))}{(\Gamma f+W)\left[4(\delta_a+\omega_{\rm MF})^2 + \Gamma^2\left(2N^2f^2Z^2 + 8N^2g^2Z^2 + f^2\right) + W^2 + 2\Gamma W\right]}, \tag{S14}$$

$$0 = \frac{1}{N}\sum_{a=1}^{N} \frac{-Z(W-\Gamma f)(2Ng(\Gamma f+W) + 2Nf(\delta_a+\omega_{\rm MF}))}{(\Gamma f+W)\left[4(\delta_a+\omega_{\rm MF})^2 + \Gamma^2\left(2N^2f^2Z^2 + 8N^2g^2Z^2 + f^2\right) + W^2 + 2\Gamma W\right]}. \tag{S15}$$

When $N \gg 1$, we can approximate the sums by integrals over the distribution of frequencies. Given a distribution of frequencies, the integrals can be evaluated numerically and $Z$ and $\omega_{\rm MF}$ can be obtained using root-finding methods. For simplicity, however, we consider a Lorenzian distribution $H(\delta) = \frac{\Delta}{\pi(\Delta^2+\delta^2)}$. In this case the integrals can be evaluated by contour integration, and we find that the order parameter $Z$ is obtained from the implicit equation

$$Z = \frac{Z\Gamma Nf(W-\Gamma f)\sqrt{\Gamma^2\left(2N^2f^2Z^2 + 8N^2g^2Z^2 + f^2\right) + W^2 + 2\Gamma fW}}{\left[2\Gamma^2N^2f^2Z^2 + (W+\Gamma f)^2\right]\left(2\Delta + \sqrt{\Gamma^2\left(2N^2f^2Z^2 + 8N^2g^2Z^2 + f^2\right) + W^2 + 2\Gamma fW}\right)}, \tag{S16}$$

while the frequency is given by

$$\omega_{\rm MF} = \frac{g(\Gamma f+W)\left(2\Delta + \sqrt{\Gamma^2\left(2N^2f^2Z^2 + 8N^2g^2Z^2 + f^2\right) + 2\Gamma fW + W^2}\right)}{2f\sqrt{\Gamma^2\left(2N^2f^2Z^2 + 8N^2g^2Z^2 + f^2\right) + 2\Gamma fW + W^2}}. \tag{S17}$$

While implicit Eq. (S16) is cumbersome, it can easily be solved with root finding methods. A simplification can be made by considering the $N \gg 1$ limit. In this case, for a given pumping $W = wN$, we obtain, to leading order in $1/N$,

$$\omega_{\rm MF} = \frac{wgN}{f}\left(1 + \frac{f\Gamma}{wN} + \frac{2\Delta}{N\sqrt{w^2 + 2f^2Z^2\Gamma^2 + 8g^2Z^2\Gamma^2}}\right), \tag{S18}$$

showing that in the thermodynamic limit the time crystal frequency is robust to heterogeneity in the oscillator detunings. If we substitute optimal order parameter $Z_{opt} = 1/\sqrt{8}$ and optimal pumping $w_{opt} = f\Gamma/2$ into (S18), we obtain

$$\omega_{\rm MF}^{opt} = \frac{wgN}{f}\left(1 + \frac{f\Gamma}{wN} + \frac{\sqrt{8}\Delta}{N\Gamma\sqrt{f^2+2g^2}}\right). \tag{S19}$$

From here we can easily see that $\delta\omega(\Delta) \sim \frac{\sqrt{8}\Delta}{N\Gamma\sqrt{f^2+2g^2}}$ at optimal pumping as discussed in the main text. In the next Section, we will compare this expression with numerically determined values from the cumulant expansion and see that there is close agreement.

Finally, we note that although here we solved for stationary rotating solutions, there can be other types of solutions, including quasiperiodic or chaotic solutions. These other possible solutions, and the bifurcations leading to them, will be explored in future research.

## III. CUMULANT EXPANSION

To obtain a model that can capture both many-body correlations and nonzero disorder, we turn to a second-order cumulant expansion, which assumes joint cumulants of order three and higher are zero, resulting in the following expansion for third-order expectations:

$$\langle\hat{\sigma}_a^\alpha\hat{\sigma}_b^\beta\hat{\sigma}_c^\gamma\rangle \approx \langle\hat{\sigma}_a^\alpha\hat{\sigma}_b^\beta\rangle\langle\hat{\sigma}_c^\gamma\rangle + \langle\hat{\sigma}_b^\beta\hat{\sigma}_c^\gamma\rangle\langle\hat{\sigma}_a^\alpha\rangle + \langle\hat{\sigma}_a^\alpha\hat{\sigma}_c^\gamma\rangle\langle\hat{\sigma}_b^\beta\rangle - 2\langle\hat{\sigma}_a^\alpha\rangle\langle\hat{\sigma}_b^\beta\rangle\langle\hat{\sigma}_c^\gamma\rangle. \tag{S20}$$

In this Section, we present the equations of motion that result, obtain results for the homogeneous system that connect the two-time correlation oscillation frequency to the mean-field frequency, compare the mean-field and cumulant frequencies for systems with nonzero disorder, and perform benchmarking of the cumulant model against exact solutions.

### A. Equations

The relevant equations of motion can be derived as:

$$\frac{d\langle\hat{\sigma}_a^+\rangle}{dt} = -i\delta_a\langle\hat{\sigma}_a^+\rangle - \frac{\Gamma f + W}{2}\langle\hat{\sigma}_a^+\rangle + \frac{\Gamma}{2}\sum_{a\neq b}(f - i2g)\langle\hat{\sigma}_a^z\hat{\sigma}_b^+\rangle, \tag{S21}$$

$$\begin{aligned}\frac{d\langle\hat{\sigma}_a^z\hat{\sigma}_b^+\rangle}{dt} =& -\left(i\delta_b + \frac{3\Gamma f + 3W}{2}\right)\langle\hat{\sigma}_a^z\hat{\sigma}_b^+\rangle - (\Gamma f - W)\langle\hat{\sigma}_b^+\rangle - \frac{\Gamma}{2}(f + i2g)\langle\hat{\sigma}_a^+\rangle - \Gamma f\langle\hat{\sigma}_a^+\hat{\sigma}_b^z\rangle \\ &+ \frac{\Gamma}{2}\sum_{j\neq a,b}(f_{bj} - i2g_{bj})\langle\hat{\sigma}_a^z\hat{\sigma}_b^z\hat{\sigma}_j^+\rangle - \Gamma\sum_{j\neq a,b}(f_{aj} + i2g_{aj})\langle\hat{\sigma}_a^+\hat{\sigma}_b^+\hat{\sigma}_j^-\rangle - \Gamma\sum_{j\neq a,b}(f_{aj} - i2g_{aj})\langle\hat{\sigma}_a^-\hat{\sigma}_b^+\hat{\sigma}_j^+\rangle\end{aligned} \tag{S22}$$

$$\frac{d\langle\hat{\sigma}_a^z\rangle}{dt} = -i\Gamma\sum_{a\neq b}2g(\langle\hat{\sigma}_a^+\hat{\sigma}_b^-\rangle - \langle\hat{\sigma}_a^-\hat{\sigma}_b^+\rangle) - \Gamma\sum_{b\neq a}f(\langle\hat{\sigma}_a^+\hat{\sigma}_b^-\rangle + \langle\hat{\sigma}_a^-\hat{\sigma}_b^+\rangle) - (\Gamma f + W)\langle\hat{\sigma}_a^z\rangle + (W - \Gamma f), \tag{S23}$$

$$\begin{aligned}\frac{d\langle\hat{\sigma}_a^+\hat{\sigma}_b^-\rangle}{dt} =& -i(\delta_a - \delta_b)\langle\hat{\sigma}_a^+\hat{\sigma}_b^-\rangle - \frac{i\Gamma}{2}g(\langle\hat{\sigma}_a^z\rangle - \langle\hat{\sigma}_b^z\rangle) + \frac{\Gamma}{2}\sum_{j\neq a,b}(f_{aj} - i2g_{aj})\langle\hat{\sigma}_a^z\hat{\sigma}_b^-\hat{\sigma}_j^+\rangle \\ &+ \frac{\Gamma}{2}\sum_{j\neq a,b}(f_{bj} + i2g_{bj})\langle\hat{\sigma}_b^z\hat{\sigma}_a^+\hat{\sigma}_j^-\rangle + \frac{\Gamma}{2}f\left(\langle\hat{\sigma}_a^z\hat{\sigma}_b^z\rangle + \frac{\langle\hat{\sigma}_a^z\rangle + \langle\hat{\sigma}_b^z\rangle}{2}\right) - (\Gamma f + W)\langle\hat{\sigma}_a^+\hat{\sigma}_b^-\rangle,\end{aligned} \tag{S24}$$

$$\begin{aligned}\frac{d\langle\hat{\sigma}_a^z\hat{\sigma}_b^z\rangle}{dt} =& -i\Gamma\sum_{j\neq a,b}2g_{aj}[\langle\hat{\sigma}_a^+\hat{\sigma}_b^z\hat{\sigma}_j^-\rangle - \langle\hat{\sigma}_a^-\hat{\sigma}_b^z\hat{\sigma}_j^+\rangle] - i\Gamma\sum_{j\neq a,b}2g_{bj}[\langle\hat{\sigma}_b^+\hat{\sigma}_a^z\hat{\sigma}_j^-\rangle - \langle\hat{\sigma}_b^-\hat{\sigma}_a^z\hat{\sigma}_j^+\rangle] \\ &- \Gamma\sum_{j\neq a,b}f_{aj}[\langle\hat{\sigma}_a^+\hat{\sigma}_b^z\hat{\sigma}_j^-\rangle + \langle\hat{\sigma}_a^-\hat{\sigma}_b^z\hat{\sigma}_j^+\rangle] - \Gamma\sum_{j\neq a,b}f_{bj}[\langle\hat{\sigma}_b^+\hat{\sigma}_a^z\hat{\sigma}_j^-\rangle + \langle\hat{\sigma}_b^-\hat{\sigma}_a^z\hat{\sigma}_j^+\rangle] \\ &+ (W - \Gamma f)(\langle\hat{\sigma}_a^z\rangle + \langle\hat{\sigma}_b^z\rangle) - 2(\Gamma f + W)\langle\hat{\sigma}_a^z\hat{\sigma}_b^z\rangle + 2\Gamma f[\langle\hat{\sigma}_a^+\hat{\sigma}_b^-\rangle + \langle\hat{\sigma}_a^-\hat{\sigma}_b^+\rangle],\end{aligned} \tag{S25}$$

$$\begin{aligned}\frac{d\langle\hat{\sigma}_a^+\hat{\sigma}_b^+\rangle}{dt} =& -i(\delta_a + \delta_b)\langle\hat{\sigma}_a^+\hat{\sigma}_b^+\rangle + \frac{\Gamma}{2}\sum_{j\neq a\neq b}(f_{aj} - i2g_{aj})\langle\hat{\sigma}_a^z\hat{\sigma}_b^+\hat{\sigma}_j^+\rangle + \frac{\Gamma}{2}\sum_{j\neq a\neq b}(f_{bj} - i2g_{bj})\langle\hat{\sigma}_b^z\hat{\sigma}_a^+\hat{\sigma}_j^+\rangle \\ &- (\Gamma f + W)\langle\hat{\sigma}_a^+\hat{\sigma}_b^+\rangle.\end{aligned} \tag{S26}$$

In these equations, $a \neq b$. Applying the cumulant expansion (S20), the above equations become closed and can be solved to obtain the dynamics. Note that this a system of equations with a size that grows as $\mathcal{O}(N^2)$.

### B. Homogeneous System

Assuming $\Delta = 0$, all dependent variables are independent of particle number. This means expectations in the above equations of motion that differ only by particle indices are equal. Taking this into consideration, we arrive at the

following system for $\langle\hat{\sigma}_a^z\rangle$, $\langle\hat{\sigma}_a^+\hat{\sigma}_b^-\rangle$, and $\langle\hat{\sigma}_a^z\hat{\sigma}_b^z\rangle$:

$$\frac{d\langle\hat{\sigma}_a^z\rangle}{dt} = -2\Gamma f(N-1)\mathrm{Re}(\langle\hat{\sigma}_a^+\hat{\sigma}_b^-\rangle) + 4\Gamma g(N-1)\mathrm{Im}(\langle\hat{\sigma}_a^+\hat{\sigma}_b^-\rangle) - \langle\hat{\sigma}_a^z\rangle(\Gamma f + W) - \Gamma f + W, \tag{S27}$$

$$\begin{aligned}\frac{d\langle\hat{\sigma}_a^+\hat{\sigma}_b^-\rangle}{dt} &= \frac{1}{2}\Gamma(N-2)(f-i2g) \\ &\left(-2\langle\hat{\sigma}_a^+\rangle\langle\hat{\sigma}_a^z\rangle\langle\hat{\sigma}_a^+\rangle^* + \langle\hat{\sigma}_a^z\hat{\sigma}_b^+\rangle\langle\hat{\sigma}_a^+\rangle^* + \langle\hat{\sigma}_a^+\rangle\langle\hat{\sigma}_a^z\hat{\sigma}_b^+\rangle^* + \langle\hat{\sigma}_a^+\hat{\sigma}_b^-\rangle^*\langle\hat{\sigma}_a^z\rangle\right) \\ &+ \frac{1}{2}\Gamma(N-2)(f+i2g) \\ &\left(-2\langle\hat{\sigma}_a^+\rangle\langle\hat{\sigma}_a^z\rangle\langle\hat{\sigma}_a^+\rangle^* + \langle\hat{\sigma}_a^z\hat{\sigma}_b^+\rangle\langle\hat{\sigma}_a^+\rangle^* + \langle\hat{\sigma}_a^+\rangle\langle\hat{\sigma}_a^z\hat{\sigma}_b^+\rangle^* + \langle\hat{\sigma}_a^+\hat{\sigma}_b^-\rangle\langle\hat{\sigma}_a^z\rangle\right) \\ &+ \frac{1}{2}\Gamma f(\langle\hat{\sigma}_a^z\rangle + \langle\hat{\sigma}_a^z\hat{\sigma}_b^z\rangle) + \langle\hat{\sigma}_a^+\hat{\sigma}_b^-\rangle(-(\Gamma f + W)),\end{aligned} \tag{S28}$$

$$\begin{aligned}\frac{d\langle\hat{\sigma}_a^z\hat{\sigma}_b^z\rangle}{dt} &= -4\Gamma(N-2)\mathrm{Re}\left((f+i2g)\left(-2\langle\hat{\sigma}_a^+\rangle\langle\hat{\sigma}_a^z\rangle\langle\hat{\sigma}_a^+\rangle^* + \langle\hat{\sigma}_a^z\hat{\sigma}_b^+\rangle\langle\hat{\sigma}_a^+\rangle^* + \langle\hat{\sigma}_a^+\rangle\langle\hat{\sigma}_a^z\hat{\sigma}_b^+\rangle^* + \langle\hat{\sigma}_a^+\hat{\sigma}_b^-\rangle\langle\hat{\sigma}_a^z\rangle\right)\right) \\ &+ 4\Gamma f\mathrm{Re}\left(\langle\hat{\sigma}_a^+\hat{\sigma}_b^-\rangle\right) + 2\langle\hat{\sigma}_a^z\rangle(W - \Gamma f) - 2\langle\hat{\sigma}_a^z\hat{\sigma}_b^z\rangle(\Gamma f + W).\end{aligned} \tag{S29}$$

We would like to determine steady state values for the various parameters. Simulations and exact solutions for small systems motivate the following ansatz:

$$\langle\hat{\sigma}_a^+\rangle = \langle\hat{\sigma}_a^z\hat{\sigma}_b^+\rangle = \langle\hat{\sigma}_a^+\hat{\sigma}_b^+\rangle = 0, \tag{S30}$$

$$\langle\hat{\sigma}_a^z\rangle = \alpha, \tag{S31}$$

$$\langle\hat{\sigma}_a^+\hat{\sigma}_b^-\rangle = \beta, \tag{S32}$$

$$\langle\hat{\sigma}_a^z\hat{\sigma}_b^z\rangle = \gamma, \tag{S33}$$

where $\alpha, \beta, \gamma$ are real and time-independent. The above system then reduces to

$$0 = -2\Gamma f(N-1)\beta - (\Gamma f + W)\alpha - \Gamma f + W, \tag{S34}$$

$$0 = \Gamma f(N-2)\alpha\beta + \frac{1}{2}\Gamma f(\alpha+\gamma) - (\Gamma f + W)\beta, \tag{S35}$$

$$0 = -4\Gamma f(N-2)\alpha\beta + 4\Gamma f\beta + 2(W - \Gamma f)\alpha - 2(\Gamma f + W)\gamma. \tag{S36}$$

This nonlinear system can be solved, giving the following steady-state values for $\langle\hat{\sigma}_a^+\hat{\sigma}_b^-\rangle$ and $\langle\hat{\sigma}_a^z\rangle$:

$$\begin{aligned}\langle\hat{\sigma}_a^+\hat{\sigma}_b^-\rangle_{SS} &= \frac{f^2\Gamma^2(2-3N) + f\Gamma(N-5)W - W^2}{4f^2\Gamma^2(N-2)(N-1)} \\ &+ \frac{\sqrt{(f^2\Gamma^2(3N-2) - f\Gamma(N-5)W + W^2)^2 - 8f^3\Gamma^3(N-2)(N-1)(f\Gamma - W)}}{4f^2\Gamma^2(N-2)(N-1)},\end{aligned} \tag{S37}$$

$$\begin{aligned}\langle\hat{\sigma}_a^z\rangle_{SS} &= \frac{f^2\Gamma^2(N+2) + f\Gamma(N+1)W + W^2}{2f\Gamma(N-2)(f\Gamma + W)} \\ &- \frac{\sqrt{(f^2\Gamma^2(3N-2) - f\Gamma(N-5)W + W^2)^2 - 8f^3\Gamma^3(N-2)(N-1)(f\Gamma - W)}}{2f\Gamma(N-2)(f\Gamma + W)}.\end{aligned} \tag{S38}$$

Again using the notation $W = wN$ and taking $N \gg 1$, Eq. (S37) simplifies to

$$\begin{aligned}\langle\hat{\sigma}_a^+\hat{\sigma}_b^-\rangle_{SS} &= -\frac{1}{4\Gamma^2 f^2}\left[w^2 - \Gamma f w\right] + \frac{1}{4\Gamma^2 f^2}\sqrt{\left[w^2 - \Gamma f w\right]^2} \\ &= -\frac{1}{4\Gamma^2 f^2} w\,(w - \Gamma f) + \frac{1}{4\Gamma^2 f^2}|w|\,|w - \Gamma f| \\ &= \begin{cases} -\frac{1}{2\Gamma^2 f^2} w\,(w - \Gamma f) & w \in [0,\, \Gamma f] \\ 0 & w > \Gamma f \end{cases}\end{aligned} \tag{S39}$$

From here we see that $w_{opt} = f\Gamma/2$ and $\langle\hat{\sigma}_a^+\hat{\sigma}_b^-\rangle_{opt} = 1/8$. Note that this is the same value for optimal pumping seen in the mean-field case in Eq. (S7) and the same optimal order parameter, noting that $Z_{opt}^2 = \langle\hat{\sigma}_a^+\hat{\sigma}_b^-\rangle_{opt} = 1/8$. Taking $N \gg 1$ in Eq. (S38) gives

$$\langle\hat{\sigma}_a^z\rangle_{SS} = \frac{1}{2f\Gamma}\left[(f\Gamma + w) - |f\Gamma - w|\right] = \frac{w}{f\Gamma}$$

where we have assumed $w < f\Gamma$ in order to be in the synchronized regime according to Eq. (S39). If we substitute in $w_{opt}$, we get $\langle\hat{\sigma}_a^z\rangle_{SS} = 1/2$. Note that the steady-state values derived above are independent of $g$. This is consistent with numerical solutions of the exact system when $\Delta = 0$. We now have a value for optimal pumping and a corresponding steady-state value for $\langle\hat{\sigma}_a^z\rangle$, which will be needed for the next section, where we determine two-time correlation decay rate and frequency.

### C. Two-time Correlation

Applying the quantum regression theorem to our equations of motion, and assuming zero disorder and particle symmetry results in the following equations for the two-time correlation function in the limit $t \to \infty$:

$$\begin{aligned}
\frac{d}{d\tau}\langle\hat{\sigma}_a^+(t+\tau)\hat{\sigma}_b^-(t)\rangle &= -\frac{\Gamma f + W}{2}\langle\hat{\sigma}_a^+(t+\tau)\hat{\sigma}_b^-(t)\rangle + \frac{\Gamma}{2}(f - i2g)\langle\hat{\sigma}_a^z(t)\rangle\langle\hat{\sigma}_a^+(t+\tau)\hat{\sigma}_a^-(t)\rangle \\
&\quad + \frac{\Gamma}{2}(f - i2g)(N-2)\langle\hat{\sigma}_a^z(t)\rangle\langle\hat{\sigma}_a^+(t+\tau)\hat{\sigma}_b^-(t)\rangle, \\
\frac{d}{d\tau}\langle\hat{\sigma}_a^+(t+\tau)\hat{\sigma}_a^-(t)\rangle &= -\frac{\Gamma f + W}{2}\langle\hat{\sigma}_a^+(t+\tau)\hat{\sigma}_a^-(t)\rangle + \frac{\Gamma}{2}(f - i2g)(N-1)\langle\hat{\sigma}_a^z(t)\rangle\langle\hat{\sigma}_a^+(t+\tau)\hat{\sigma}_b^-(t)\rangle,
\end{aligned}$$

where we distinguish between diagonal and off-diagonal correlation functions with the subscripts, but no longer particle number, so this is simply a linear system of two equations with the matrix

$$\begin{pmatrix} -\frac{\Gamma f+W}{2} + \frac{\Gamma}{2}(f-i2g)(N-2)\langle\hat{\sigma}_a^z\rangle_{SS} & \frac{\Gamma}{2}(f-i2g)\langle\hat{\sigma}_a^z\rangle_{SS} \\ \frac{\Gamma}{2}(f-i2g)(N-1)\langle\hat{\sigma}_a^z\rangle_{SS} & -\frac{\Gamma f+W}{2} \end{pmatrix},$$

where we have used $\lim_{t\to\infty}\langle\hat{\sigma}_a^z(t)\rangle = \langle\hat{\sigma}_a^z\rangle_{SS}$. Inserting the steady-state value $\langle\hat{\sigma}_a^z\rangle_{SS} = w/\Gamma f$, the eigenvalues are:

$$\begin{aligned}
\lambda_1 &= -\frac{w(N+1) + f\Gamma}{2} + i\frac{wg}{f}, \\
\lambda_2 &= -\frac{w + f\Gamma}{2} - i\frac{wg}{f}(N-1).
\end{aligned}$$

The real parts of these eigenvalues determine the decay rate of the two-time correlation function. Note that $\mathrm{Re}(\lambda_1)$ is negative and scales linearly with $N$, so it will cause rapid decay and the corresponding mode will not contribute meaningfully to oscillations in the thermodynamic limit. In contrast, the real part of $\lambda_2$ is independent of $N$, so oscillation frequency for large $N$ will be determined by its imaginary part. This will be, for $N \gg 1$,

$$\omega_C = \frac{wgN}{f},$$

which agrees with the mean-field estimate to leading order in $1/N$. Note also that the real part of $\lambda_2$ is proportional to $f\Gamma$ at optimal pumping, and therefore so is the decay rate. We also notice, however, that the decay is independent of $g$. This is not, as we have seen, in agreement with the exact solution. This constrains the window in $g$ where the cumulant can be applied to small values, as disparity in decay rate is small in this regime as we will see below. For all numerically derived results, spectral width $B$ is used as a proxy for the decay rate given here by $|\mathrm{Re}[\lambda_2]|$. The value of $B$ is calculated as the full-width-at-half-max (FWHM) of the discrete Fourier transform of the numerically determined solution.

### D. Disorder

Allowing $\Delta > 0$, we can solve for the two-time correlation function numerically and examine its frequency. Fig. S1 compares this frequency to the derived mean-field value seen in Eq. (S19) where pumping and synchronization are assumed to be optimal and $N = 100$. As can be seen, there is close agreement, and the two values remain close as $\Delta$ increases. It should be noted that for our simulations, we take the $\{\delta_a\}_{a=1}^N$ to be spaced at intervals of equal probability according to the Lorentzian probability density function to ensure a zero mean.

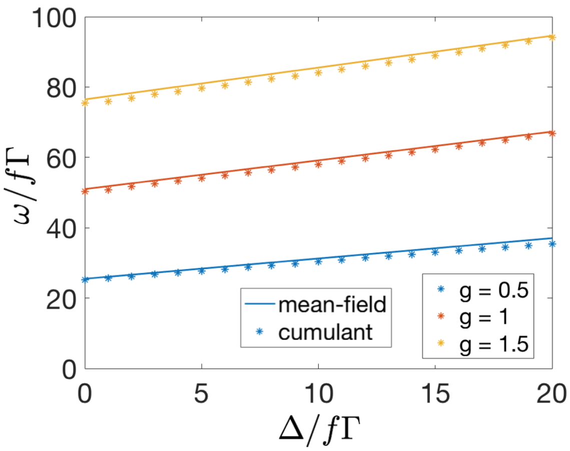


FIG. S1. Comparison of numerically determined cumulant two-time correlation frequency (symbols) and predicted mean-field frequency (solid lines) at optimal pumping when $N = 100$

### E. Benchmarking

Fig. S2 compares the cumulant expansion solution to that of the exact solver in two cases where the exact solution is accessible. In the left panel, we compare the order parameter $Z_Q$ of the synchronized system in the case where the number of particles is small. In the right panel, we compare the real part of the two-time correlation function $C(\tau)$ for a larger system without disorder. In both cases, we see close agreement between the cumulant expansion and the exact solution.

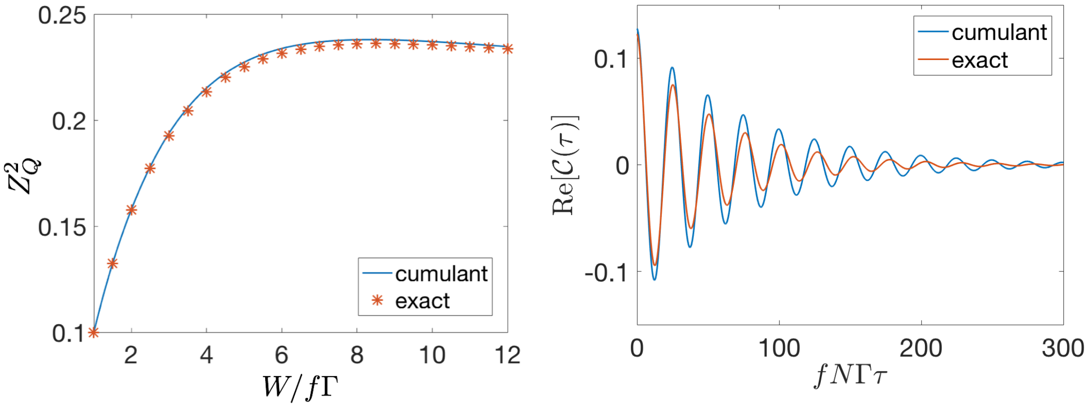


FIG. S2. Comparing the cumulant expansion solution against the exact solver for the order parameter when $N = 5$, $f = 1$, $g = 0.5$, $\Delta = 1$ for a range of $W/f\Gamma$ (left panel) and for $\mathrm{Re}[C(\tau)]$ where $N = 100$, $f = 1$, $g = 0.5$, $\Delta = 0$, and optimal $W$ (right panel)

## IV. MUTUAL INFORMATION

To gain insight into the growth of mutual information in the transient dynamics, we derive an expression for the derivative of the two particle mutual information for zero disorder at small times up to first-order in $t$. To do this, we write each of the necessary density operators, $\hat{\rho}_{AB}$, $\hat{\rho}_A$, and $\hat{\rho}_B$, in the Pauli basis according to

$$\hat{\rho} = \frac{1}{2^M}\sum_{\vec{\alpha}} c_{\vec{\alpha}}\hat{\rho}_{\vec{\alpha}}, \quad \hat{\rho}_{\vec{\alpha}} \equiv \bigotimes_{j=1}^{M} \hat{\sigma}^{\alpha_j},$$

where $\hat{\sigma}^{\alpha_j} \in \{\mathbb{1}, \hat{\sigma}^+, \hat{\sigma}^-, \hat{\sigma}^z\}$ and $M$ is the number of particles in the subsystem, e.g. $M = 2$ in the case of $\hat{\rho}_{AB}$. Note that $c_{\vec{\alpha}} = \mathrm{Tr}[\hat{\rho}\hat{\rho}_{\vec{\alpha}}] = \langle \hat{\rho}_{\vec{\alpha}} \rangle$, thus we can write $\hat{\rho}_{AB}$ in terms of second-order expectations of Pauli operators, and $\hat{\rho}_A$ and $\hat{\rho}_B$ in terms of first-order expectations. We then expand each density operator to second order in $t$ according to,

$$\hat{\rho}(t) \approx \hat{\rho}\Big|_{t=0} + t\partial_t \hat{\rho}\Big|_{t=0} + \frac{t^2}{2}\partial_{tt}\hat{\rho}\Big|_{t=0}, \tag{S40}$$

using the cumulant equations when $\Delta = 0$ to expand the derivatives of expectations of Pauli operators to be in terms of the expectations of the operators themselves. This allows for evaluation at $t = 0$. Eigenvalues can then be determined using first-order perturbation theory. Note that particle symmetry when $\Delta = 0$ ensures that expressions derived for eigenvalues of $\hat{\rho}_{AB}$, $\hat{\rho}_A$, and $\hat{\rho}_B$ are the same for any choice of $A$ and $B$. The initial condition is taken such that all particles are spin up in the $\hat{x}$-direction at $t = 0$. This approach results in the following expression for the mutual information derivative at small times:

$$\begin{aligned}\frac{dI_{AB}}{dt} = & \frac{1}{4}\left[-2(f\Gamma + W)\log\left[t(f\Gamma + W)\right] + (2f\Gamma + W)\log\left[t(2f\Gamma + W)\right] + W\log(tW)\right] \\ & + \left[\frac{\Gamma^2}{2}\left(-2f^2 - 4g^2\right) + W\log\left(tW\right)\left(f\Gamma(N+2) - 3W\right)\right. \\ & + \log\left[t\left(f\Gamma + W\right)\right]\left(\Gamma^2\left(f^2\left(-\left(N^2 - 2\right)\right) - 4g^2(N-1)\right) + 2f\Gamma NW + W^2\right) \\ & + \log\left[t\left(2f\Gamma + W\right)\right]\left(\Gamma^2\left(f^2\left(N^2 - 5\right) + 4g^2(N-2)\right) - f\Gamma(3N+4)W + W^2\right) \\ & \left. + \frac{1}{2}\left(\Gamma^2\left(3f^2 + 4g^2\right) + 2f\Gamma W + W^2\right)\log\left[t^2\left(\Gamma^2\left(3f^2 + 4g^2\right) + 2f\Gamma W + W^2\right)\right]\right]\frac{t}{4} + \mathcal{O}(t^2).\end{aligned} \tag{S41}$$

Note that the $t$ in the arguments of the logarithms will cancel and they are in the above expression only for dimensional consistency. The approximation for the density operators in (S40) will have an error term that is to the same order in $t$ and $N$. This imposes the restriction $f\Gamma t \ll 1/N$. This works well for our purposes, since we are interested in characteristic time scales of the time crystal oscillations which, as we have seen from $\omega_{\mathrm{MF}}$ and $\omega_{\mathrm{C}}$, have a frequency that grows linearly with $N$ to leading order. Using the change of variables $\eta \equiv fN\Gamma t$ where $\eta \ll 1$, going to first order in time, and expanding to leading order for large $N$, Eq. (S41) becomes

$$\frac{dI_{AB}}{dt} \approx \frac{f^2\Gamma^2}{4Nw} + \left(-\frac{3f^3\Gamma^3}{8Nw^2} + \frac{5f^2\Gamma^2}{4Nw} - \frac{9f\Gamma}{4N} + \frac{g^2\Gamma^2}{Nw} + \frac{(f\Gamma - 2w)^2}{4w}\right)\eta + \mathcal{O}\left(\frac{1}{N^2}\right). \tag{S42}$$

Note that this vanishes in the thermodynamic limit only when pumping is optimal, i.e. $w = f\Gamma/2$. At this value of pumping, we get

$$\frac{dI_{AB}}{dt} \approx \frac{f\Gamma}{2}\left(\frac{1}{N} + \left(\frac{4g^2}{f^2} - \frac{5}{2}\right)\frac{\eta}{N}\right) + \mathcal{O}\left(\frac{1}{N^2}\right),$$

thus leading to constant $dI_{AB}/dt$ contours of $g/f \lesssim \sqrt{N}$ as noted in the main text. Using optimal pumping, $\Gamma = f = 1$, $\eta = 0.03$, and plotting $1/I'_{AB}(\eta)$ over a range of $g$ and $N$ produces the contour plot found in Fig. 2 of the main text. Large values correspond to regions of slow growth in mutual information while small values indicate rapid growth on time scales characteristic of the time crystal oscillations. Extending our analysis using second order perturbation theory produces a result that is very similar at optimal pumping, but includes a correction term on the order of $\eta\log(\eta)/N$ with a coefficient of the same order in $g$. This reduces the error of the approximation with increasing $g$ to a point where it is very small over the parameter regime of interest without changing the broader analysis given above.

For a small system, we can draw a connection between the growth of mutual information and the eigenvalues of the Liouvillian $L$ given by the master equation (S1) which has the form $\partial_t\hat{\rho} = L[\hat{\rho}]$. To examine frequencies, we restrict our attention to the lowest lying eigenvalues of $L$ with nonzero imaginary part. Also, since we are looking for contributors to two-time correlation frequency, we consider only those eigenvalues with eigenvectors that are not orthogonal to $\lim_{t\to\infty} S^-\hat{\rho}(t)$, which is what the operator $e^{L\tau}$ operates on in the quantum regression formula. Fig. S3 plots the imaginary part of these eigenvalues for a system at optimal pumping where $N = 5$. The blue line is a linear fit of the numerically determined frequency of the two-time correlation function $\mathcal{C}(\tau)$. As expected, the imaginary parts of the eigenvalues align closely with this frequency, particularly for small $g/f$. In panel (a), the color gives the magnitude of the real part of the Liouvillian eigenvalues, which determines the decay rate of $\mathcal{C}(\tau)$ for the corresponding frequency mode. As can be seen, this decay is gradual for small $g/f$ and increases with this parameter. In panel (b), the color gives the derivative of two particle mutual information at $\eta = 0.03$ in the transient dynamics starting at spin up in the $\hat{x}$-direction. Note that the increase in decay rate aligns closely with the increase in mutual information as we vary $g/f$.

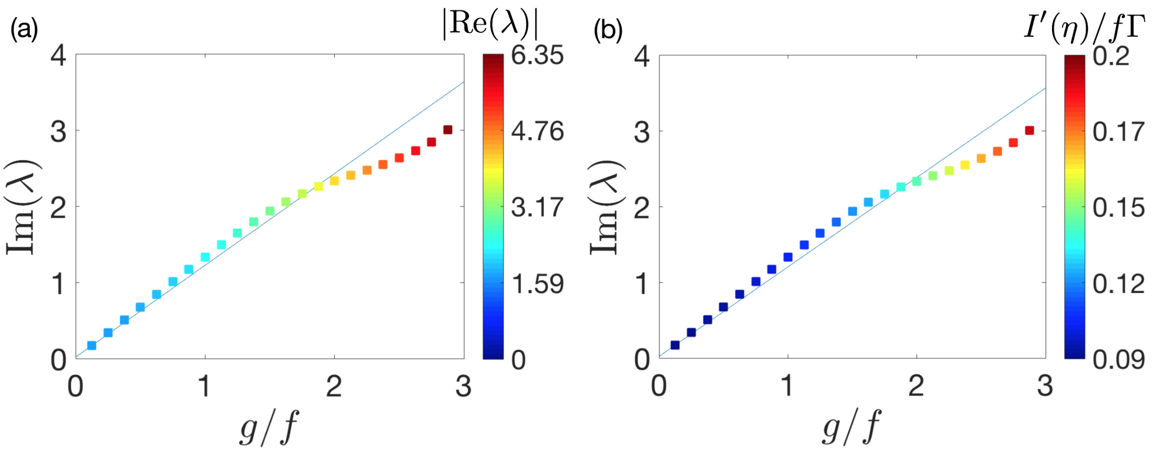


FIG. S3. Imaginary part of the Liouvillian eigenvalue versus $g/f$ plotted with a linear fit of the numerically determined frequency of $\mathcal{C}(\tau)$ (blue). In panel (a), color corresponds to the magnitude of the eigenvalue real part and in panel (b) it corresponds to the mutual information derivative at $\eta = 0.03$ in the transient dynamics

[S1] H. Sakaguchi and Y. Kuramoto, Progress of Theoretical Physics **76**, 576 (1986).
[S2] B. Zhu, J. Schachenmayer, M. Xu, F. Herrera, J. G. Restrepo, M. J. Holland, and A. M. Rey, New Journal of Physics **17**, 083063 (2015).
